# Supplementary material for: Effect of Localization on Photoluminescence and Zero-Field Splitting of Silicon Color Centers
Source: arXiv:2206.04824 ancillary file (2022-09-23)
Supplement: Supplementary file 1 [file Supplemental_Materials.pdf]

# Supplementary Material: Computational Characterization of Silicon Defect Centers


Vsevolod Ivanov[1,2], Jacopo Simoni[2], Yeonghun Lee[2,4], Wei Liu[1], Kaushalya Jhuria[1], Walid Redjem[3], Yertay Zhiyenbayev[3], Christos Papapanos[3], Wayesh Qarony[3], Boubacar Kante[1,3], Arun Persaud[1], Thomas Schenkel[1], and Liang Z. Tan[2]

[1]Accelerator Technology and Applied Physics Division, Lawrence Berkeley National Laboratory, Berkeley, CA 94720, USA
[2]Molecular Foundry, Lawrence Berkeley National Laboratory, Berkeley, CA 94720, USA
[3]Department of Electrical Engineering and Computer Sciences, University of California, Berkeley, CA 94720, USA
[4]Department of Electronics Engineering, Incheon National University, Incheon 22012, Republic of Korea


## Supplementary Note 1: Additional Details for Photoluminescence calculation

In order to calculate the photoluminescence spectra of the quantum defect centers, we employ the generating function approach [S1]. Within this method the optical spectral function is directly obtained from the generating function $G(t) = e^{S(t)-S(0)}$ of the electron-phonon spectral function $S(\hbar\omega)$ given by

$$S(\hbar\omega) = \sum_{\mathbf{q}\in\mathrm{BZ}} \sum_{\lambda} \frac{\omega_\lambda(\mathbf{q}) f_\lambda(\mathbf{q})^2}{2\hbar} \delta(\hbar\omega - \hbar\omega_\lambda(\mathbf{q}))\,, \tag{S1}$$

$$S(t) = \int_0^\infty S(\hbar\omega) e^{-i\omega t} d(\hbar\omega) \tag{S2}$$

where $\hbar\omega_\lambda(\mathbf{q})$ is the phonon energy of the mode $\lambda$ and wave vector $\mathbf{q}$, and the coefficients $f_\lambda(\mathbf{q})$ are given by

$$f_\lambda(\mathbf{q}) = \sum_{\alpha i} m_\alpha^{1/2} (R_{e,\alpha i} - R_{g,\alpha i}) \varepsilon_\lambda^{\alpha i}(\mathbf{q})\,, \tag{S3}$$

$\alpha$ and $i$ indicate respectively the atom and direction component index, $\varepsilon_\lambda^{\alpha i}(\mathbf{q})$ is the coefficient of the $\lambda$ phonon eigenvector, $m_\alpha$ is the atom mass and $\mathbf{R}_e$, $\mathbf{R}_g$ are the atomic coordinates in the excited and ground state configurations. The optical spectral function S2 is then computed from the Fourier transform of $G(t)$

$$A(E_{\mathrm{ZPL}} - \hbar\omega) = \frac{1}{2\pi} \int_{-\infty}^{\infty} G(t) e^{i\omega t - \gamma|t|} dt\,, \tag{S4}$$

where the broadening $\gamma$ is set for all the defects to $\gamma = 1\,meV$ in order to reproduce as close as possible the experimental data available for B and W centers[]. All the atomic structures are relaxed in VASP in their ground and excited state configurations. The phonon eigenvectors and eigenvalues are obtained from *phonopy*[] in the relaxed ground state configuration of the defect. We use a $\mathbf{q}$-points grid of size $22 \times 22 \times 22$.

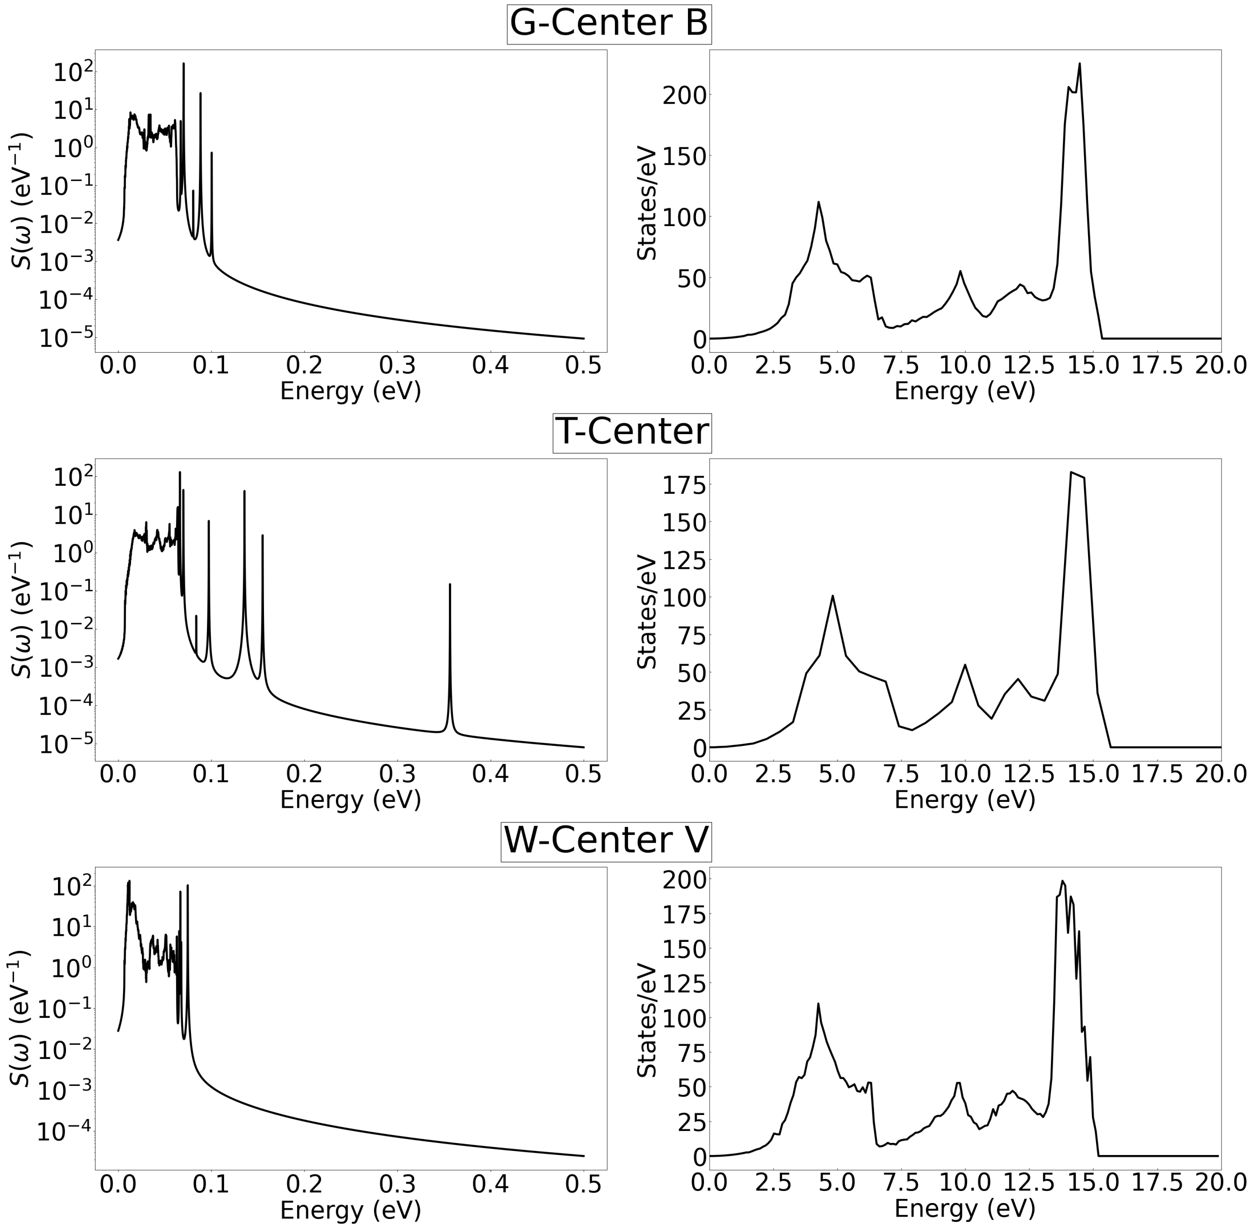


Figure S1: Electron-phonon spectral function (left) and phonon density of states (right) for the G-center, T-center, W-center.

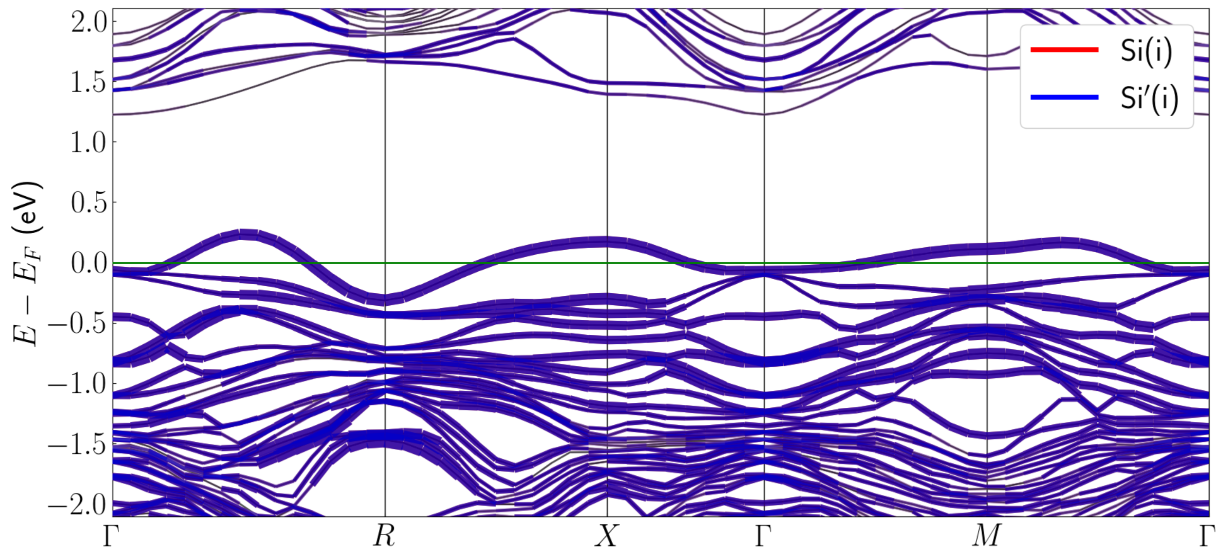


Figure S2: Atom-projected band structure of the W-center, with contributions from the two different types of Si atoms of the six total interstitials comprising the defect indicated in red and blue respectively.

## Supplementary Note 2: Tight-binding model for G-center defect states

Here we explicitly show the tight-binding Hamiltonians used in the derivation of the G-center defect energy levels. The two configurations, G-center Type A and G-center Type B, can be understood in terms of the bond orders of the atoms in the defect center. For G-center Type A, both the substitutional silicon $\mathrm{Si}_{(s)}$ and interstitial carbon $\mathrm{C}_{(i)}$ have three nearest neighbor bonds with approximately $sp^2$ hybridization. We can consider a nearest neighbor tight binding model that includes on $\mathrm{C}_{(i)}$ the $p_z$ orbital as well as three $sp_1^2$, $sp_2^2$, $sp_3^2$ orbitals, which are connected to the nearest three Si atoms by hoppings $t$. Setting the energy of the $p_z$ orbital to be $\epsilon_0 = 0$, we can take $\Delta\epsilon_1$ to be the energy of the $sp^2$, and $\Delta\epsilon_2$ to be the energy of the bonding orbitals on the nearest Si atoms. The Hamiltonian can explicitly be written

$$\mathcal{H}_{(sp^2)} = \begin{bmatrix} \epsilon_0^C & 0 & 0 & 0 & 0 & 0 & 0 \\ 0 & \Delta\epsilon_1 & 0 & 0 & t & 0 & 0 \\ 0 & 0 & \Delta\epsilon_1 & 0 & 0 & t & 0 \\ 0 & 0 & 0 & \Delta\epsilon_1 & 0 & 0 & t \\ 0 & t & 0 & 0 & \Delta\epsilon_2 & 0 & 0 \\ 0 & 0 & t & 0 & 0 & \Delta\epsilon_2 & 0 \\ 0 & 0 & 0 & t & 0 & 0 & \Delta\epsilon_2 \end{bmatrix} \tag{S5}$$

Diagonalizing yields the following eigenvalues – the defect level at $E_{\mathrm{C}(i)} = \epsilon_0^C = 0$, as well as two sets of triply degenerate levels $E_\pm = (1/2)\left(\Delta\epsilon_1 + \Delta\epsilon_2 \pm \sqrt{(\Delta\epsilon_1 - \Delta\epsilon_2)^2 + 4t^2}\right)$. The hopping exceeds the separation between the orbital energies $t >> (\Delta\epsilon_1 - \Delta\epsilon_2)$, so these states have energies $E_\pm \sim (\Delta\epsilon_1 + \Delta\epsilon_2)/2 \pm t$, forming a gap $\Delta \sim 2t$ which contains the defect level. A similar argument can be made for the substitutional silicon $\mathrm{Si}_{(s)}$, which will also have two sets of three levels separated by a gap $\Delta \sim 2t$ which contains the defect level from the Si $p_z$ orbital at $E_{\mathrm{Si}(s)} = \epsilon_0^{Si}$. However, the triple degeneracy of those non-defect levels will be lifted since two of the bonding atoms are carbon and the third is silicon.

This explains how for the G-center Type A, the non-bonding $p$-orbitals of $\mathrm{Si}_{(s)}$ and $\mathrm{C}_{(i)}$ form the defect levels of the system. The remaining states, along with the states from the tetrahedrally bonded Si atoms of the crystal, form the valence and conduction bands. In fact, in G-center Type B, the carbon atom moves to the substitutional position, $\mathrm{C}_{(s)}$, effectively becoming tetrahedrally bonded. We can diagonalize the Hamiltonian of this $sp^3$-hybridized system to see that it does not contribute to the defect levels. The Hamiltonian

$$\mathcal{H}_{(sp^3)} = \begin{bmatrix} \Delta\epsilon_1 & 0 & 0 & 0 & t & 0 & 0 & 0 \\ 0 & \Delta\epsilon_1 & 0 & 0 & 0 & t & 0 & 0 \\ 0 & 0 & \Delta\epsilon_1 & 0 & 0 & 0 & t & 0 \\ 0 & 0 & 0 & \Delta\epsilon_1 & 0 & 0 & 0 & t \\ t & 0 & 0 & 0 & \Delta\epsilon_2 & 0 & 0 & 0 \\ 0 & t & 0 & 0 & 0 & \Delta\epsilon_2 & 0 & 0 \\ 0 & 0 & t & 0 & 0 & 0 & \Delta\epsilon_2 & 0 \\ 0 & 0 & 0 & t & 0 & 0 & 0 & \Delta\epsilon_2 \end{bmatrix} \tag{S6}$$

has eigenvalues $E_\pm = (1/2)\left(\Delta\epsilon_1 + \Delta\epsilon_2 \pm \sqrt{(\Delta\epsilon_1 - \Delta\epsilon_2)^2 + 4t^2}\right)$ which form two quadruply degenerate sets separated by $\Delta = 2t$. On the other hand, the silicon in the G-center Type B moves to the interstitial position, $\mathrm{Si}_{(i)}$ and has only two bonds to nearby carbon atoms. Due to the bent configuration of the $\mathrm{C}_{(s)}$-$\mathrm{Si}_{(i)}$-$\mathrm{C}_{(s)}$ chain, the $sp^2$ hybridization is still appropriate, with only two of the $sp^2$ orbitals participating in bonding. The Hamiltonian can be written

$$\mathcal{H}_{(sp^2)} = \begin{bmatrix} \epsilon_0^S & 0 & 0 & 0 & 0 & 0 \\ 0 & \Delta\epsilon_1 & 0 & 0 & t & 0 \\ 0 & 0 & \Delta\epsilon_1 & 0 & 0 & t \\ 0 & 0 & 0 & \Delta\epsilon_1 & 0 & 0 \\ 0 & t & 0 & 0 & \Delta\epsilon_2 & 0 \\ 0 & 0 & t & 0 & 0 & \Delta\epsilon_2 \end{bmatrix}. \tag{S7}$$

In this case there are two doubly degenerate pairs with eigenvalues $E_\pm = (1/2)\left(\Delta\epsilon_1 + \Delta\epsilon_2 \pm \sqrt{(\Delta\epsilon_1 - \Delta\epsilon_2)^2 + 4t^2}\right)$, as well as two defect levels in the gap with energies $E^1_{\mathrm{S}(i)} = \epsilon_0^S = 0$ and $E^2_{\mathrm{S}(i)} = \Delta\epsilon_1$, corresponding to the non-bonding $p_z$ and $sp^2$ orbitals on the interstitial silicon.

## Supplementary Note 3: Sample preparation details for experimental data in Figure 4

**G-center** — The sample was silicon on insulator (SOI), ⟨100⟩, with a device layer thickness of 230 nm. The sample had been implanted with carbon ions, 4x1013 $cm^{-2}$, at 36 keV, under an angle of 7°, and was annealed at 1000 °C for 7 s in $N_2$. All color center photoluminescence measurements where conducted at a temperature of 4 K [S4].

**T-center** — The sample was prepared on SOI ⟨100⟩ wafer, with a device layer thickness of 220 nm and an oxide layer thickness of 2 $\mu$m. The sample preparation was as follows: (1) implantation with Carbon ions having energy 38 keV, 1013 $cm^{-2}$ ; (2) rapid annealing at 1000 °C for 20 s in $N_2$: (3) implantation with hydrogen ions having energy 9 keV, 1013 cm-2; (4) Boiling in deionized water for 1 hour at a hotplate temperature around 180 °C; (5) 3 minutes of annealing at 420 °C. Photoluminescence measurements were performed at a temperature of 4 K [S2].

**W-center** — The sample was silicon ⟨111⟩ . The sample was exposed to two pulses of laser-accelerated ions, which led to the direct formation of W centers without thermal annealing [S3]. A small contribution from G-centers is also visible in the spectrum at 1279 nm.

## Supplementary Note 4: Zero-field splitting convergence

Convergence of the Zero-Field Splitting was checked using $1 \times 1 \times 1$, $1 \times 1 \times 2$, and $1 \times 2 \times 2$ k-point grids. Figure S3 shows that the values remain relatively stable as the grid increases, meaning that the Γ-point grids used in the manuscript only slightly underestimate the value of the ZFS.

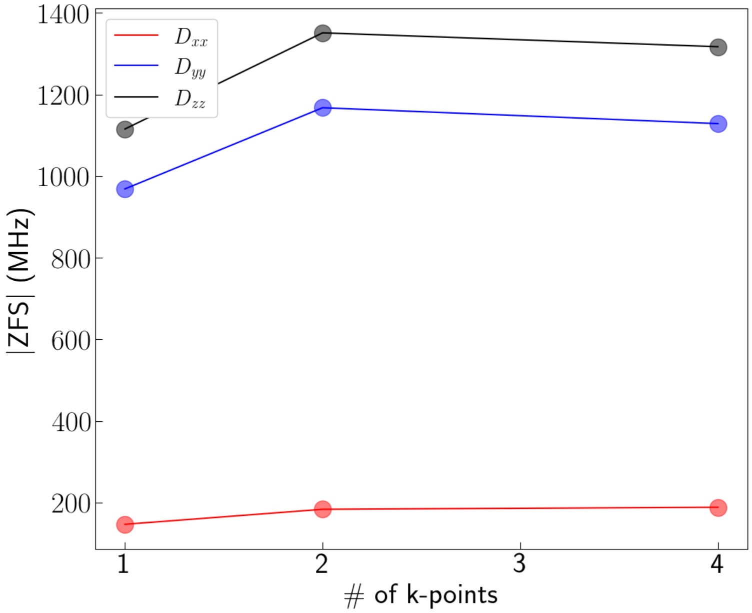


Figure S3: Diagonal of the ZFS tensor of the excited triplet state of the G-center as a function of increasing number of k-points

## Supplementary Note 5: Enhancement of the ZFS using Tight-binding-derived orbitals

For a two particle system, the ZFS integral can be written as

$$D_{zz} = -\frac{\mu_0 g^2 \mu_B^2}{4\pi} \iint \rho(\boldsymbol{R}_1, \boldsymbol{R}_2) \frac{R^2 - 3z^2}{R^5} d\boldsymbol{R}_1 d\boldsymbol{R}_2, \tag{1}$$

where $R = |\boldsymbol{R}_2 - \boldsymbol{R}_1|$, and $\rho(\boldsymbol{R}_1, \boldsymbol{R}_2) = |\Psi(\boldsymbol{R}_1, \boldsymbol{R}_2)|^2$ is the two-particle density. The two-particle wavefunction can be approximated as the antisymmetric product of the single particle states, $\Psi = [\psi_i(\boldsymbol{R}_1)\psi_j(\boldsymbol{R}_2) - \psi_i(\boldsymbol{R}_2)\psi_j(\boldsymbol{R}_1)]/\sqrt{2}$. Here $i$ and $j$ indices denote the single-electron states involved – Si($p_z$) and C($p_z$) for GCA, or Si($p_z$) and Si($sp_1^2$) for GCB. For GCA and GCB, the two electron wavefunctions can be written using the defect states derived from the tight-binding model above:

$$\Psi^{\mathrm{GCA}} = \frac{1}{\sqrt{2}} \left[ \psi_{p_z}^{\mathrm{Si}}(\boldsymbol{R}_1) \psi_{p_z}^{\mathrm{C}}(\boldsymbol{R}_2) - \psi_{p_z}^{\mathrm{Si}}(\boldsymbol{R}_2) \psi_{p_z}^{\mathrm{C}}(\boldsymbol{R}_1) \right] \tag{2}$$

$$\Psi^{\mathrm{GCB}} = \frac{1}{\sqrt{2}} \left[ \psi_{p_z}^{\mathrm{Si}}(\boldsymbol{R}_1) \psi_{sp_1^2}^{\mathrm{Si}}(\boldsymbol{R}_2) - \psi_{p_z}^{\mathrm{Si}}(\boldsymbol{R}_2) \psi_{sp_1^2}^{\mathrm{Si}}(\boldsymbol{R}_1) \right] \tag{3}$$

Using these expressions for the two-electron defect states, the $D_{zz}$ component of the ZFS can be expressed as $D_{zz}^{ij} = (J^{ij} + K^{ij})/2$, where

$$J^{ij} = \iint \psi_i(\boldsymbol{R}_1)\psi_j(\boldsymbol{R}_2) \frac{R^2 - 3z^2}{R^5} \psi_i^*(\boldsymbol{R}_1)\psi_j^*(\boldsymbol{R}_2) d\boldsymbol{R}_1 d\boldsymbol{R}_2 \tag{4}$$

$$K^{ij} = \iint \psi_i(\boldsymbol{R}_1)\psi_j(\boldsymbol{R}_2) \frac{R^2 - 3z^2}{R^5} \psi_i^*(\boldsymbol{R}_2)\psi_j^*(\boldsymbol{R}_1) d\boldsymbol{R}_1 d\boldsymbol{R}_2. \tag{5}$$

For both G-center structures, the above expressions may be simplified by choosing an appropriate coordinate system. For GCA, the natural choice is to align the defect orbital on Si with the $z$-axis, the defect orbital on $\mathrm{C}_{(i)}$ with the $y$-axis, so that the bond vector $\boldsymbol{d} = (d, 0, 0)$ is aligned along the $x$-direction. After transforming into the local coordinates of each atom, $\boldsymbol{R}_1, \boldsymbol{R}_2 \to \boldsymbol{r}_1, \boldsymbol{r}_2 + \boldsymbol{d}$, the integral $J^{ij}$ above becomes

$$\iint p_z^2(\boldsymbol{r}_1) p_y^2(\boldsymbol{r}_2) \frac{|\boldsymbol{r}_2 - \boldsymbol{r}_1 + \boldsymbol{d}|^2 - |z_1 - z_2|^2}{|\boldsymbol{r}_2 - \boldsymbol{r}_1 + \boldsymbol{d}|^5} d\boldsymbol{r}_1 d\boldsymbol{r}_2, \tag{6}$$

with the integral for $K^{ij}$ acquiring a similar form. In the limit $|\boldsymbol{r}_2 - \boldsymbol{r}_1| \ll \boldsymbol{d}$, the integral above will reduce to $C/d^3$, where $C$ is the factor arising from the integrals over $\boldsymbol{r}_1, \boldsymbol{r}_2$. Thus for G-center A, where the defect states are localized to separate atoms, $D_{zz}$ will have the above form and scale as $1/d^3$, resulting in a much smaller ZFS than for G-center B, where the defect orbitals are localized to the same atom.

# References


[S1] Audrius Alkauskas, Bob B Buckley, David D Awschalom, and Chris G Van de Walle. First-principles theory of the luminescence lineshape for the triplet transition in diamond NV centres. *New Journal of Physics*, 16(7):073026, jul 2014.

[S2] Jiahui Huang, Murat Can Sarihan, Jin Ho Kang, Baolai Liang, Wei Liu, and Chee Wei Wong. Cryogenic optical transitions of t centers in bulk silicon and silicon-on-insulator for cavity quantum electrodynamics. In *Frontiers in Optics + Laser Science 2021*, page JTu7A.2. Optica Publishing Group, 2021.

[S3] Walid Redjem, Ariel J. Amsellem, Frances I. Allen, Gabriele Benndorf, Jianhui Bin, Stepan Bulanov, Eric Esarey, Leonard C. Feldman, Javier Ferrer Fernandez, Javier Garcia Lopez, Laura Geulig, Cameron R. Geddes, Hussein Hijazi, Qing Ji, Vsevolod Ivanov, Boubacar Kante, Anthony Gonsalves, Jan Meijer, Kei Nakamura, Arun Persaud, Ian Pong, Lieselotte Obst-Huebl, Peter A. Seidl, Jacopo Simoni, Carl Schroeder, Sven Steinke, Liang Z. Tan, Ralf Wunderlich, Brian Wynne, and Thomas Schenkel. Defect engineering of silicon with ion pulses from laser acceleration, 2022.

[S4] Thomas Schenkel, Walid Redjem, Arun Persaud, Wei Liu, Peter A. Seidl, Ariel J. Amsellem, Boubacar Kanté, and Qing Ji. Exploration of defect dynamics and color center qubit synthesis with pulsed ion beams. *Quantum Beam Science*, 6(1), 2022.
